# Supplementary material for: Machine Learning-Aided First-Principles Calculations of Redox Potentials
Source: arXiv:2309.13217 ancillary file (2024-03-22)
Supplement: Supplementary file 1 [file supplementary_information.pdf]

# Supplementary Information for Machine Learning-Aided First-Principles Calculations of Redox Potentials

Ryosuke Jinnouchi

*Toyota Central Research and Developments Laboratories Inc.* *

Ferenc Karsai

*VASP Software GmbH/Sensengasse 8, 1090 Vienna, Austria*

Georg Kresse†

*Computational Materials Physics, Faculty of Physics,*

*University of Vienna, 1090 Vienna, Austria*

(Dated: March 23, 2024)

* e1262@mosk.tytlabs.co.jp

† Also at VASP Software GmbH.

## S1. SUPPLEMENTARY DATA OF MLFF AND Δ-ML

The parameter sets for the descriptors and kernel basis functions for bulk and slab systems are summarized in Table S1. The number of structures calculated using the FP method to generate training data for the MLFFs is presented in Table S2. The probability densities for finding specific differences in potential energy and force between the ML and FP results are summarized in Figures S1, S2, S3, and S4 for the 128$H_2O$ slab, $Fe^{3+}$/$Fe^{2+}$+64$H_2O$ bulk solutions, $Cu^{2+}$/$Cu^{+}$+64$H_2O$ bulk solutions, and $Ag^{2+}$/$Ag^{+}$+64$H_2O$ bulk solutions, respectively. In the error analysis of the MLFF models, a 100 ps NVT-ensemble MD simulation at 298.15 K was conducted for each system using the MLFF model. From each trajectory, 100 structures were randomly selected, and FP calculations using the RPBE+D3 functional were performed. In the error analysis of the Δ-ML models, 360 structures for the $Fe^{3+}$/$Fe^{2+}$ system and 160 structures for each of the $Cu^{2+}$/$Cu^{+}$ and $Ag^{2+}$/$Ag^{+}$ systems were randomly selected from the trajectories. For the selected trajectories, FP calculations using hybrid functionals were conducted. The probability density indicates that Δ-ML models achieve an error reduction exceeding an order of magnitude in comparison to the MLFF models.

Table S 1. Parameter sets of descriptors and kernel basis functions for bulk and slab systems.

| | | | | | | | | | | | |
|---|---|---|---|---|---|---|---|---|---|---|---|
| Parameters for bulk systems | | | | | | | | | | | |
| $\zeta$ | 4 | $\beta^{(3)}$ | 1.0 | $R_{\mathrm{cut}}^{(3)}$ | 5.0 | $\sigma_{\mathrm{atom}}^{(3)}$ | 0.5 | $N_{\mathrm{R}}^{(3)}$ | 10 | $L_{\mathrm{max}}^{(3)}$ | 4 |
| Parameters for water slab | | | | | | | | | | | |
| $\zeta$ | 4 | $\beta^{(2)}$ | 0.5 | $R_{\mathrm{cut}}^{(2)}$ | 8.0 | $\sigma_{\mathrm{atom}}^{(2)}$ | 0.5 | $N_{\mathrm{R}}^{(2)}$ | 12 | | |
| | | $\beta^{(3)}$ | 0.5 | $R_{\mathrm{cut}}^{(3)}$ | 4.0 | $\sigma_{\mathrm{atom}}^{(3)}$ | 0.5 | $N_{\mathrm{R}}^{(3)}$ | 6 | $L_{\mathrm{max}}^{(3)}$ | 4 |

Table S 2. The numbers of structures $N_{\mathrm{st}}$ calculated by the FP method to generate training data for the MLFFs.

| System | $N_{\mathrm{st}}$ | System | $N_{\mathrm{st}}$ | System | $N_{\mathrm{st}}$ | System | $N_{\mathrm{st}}$ |
|---|---|---|---|---|---|---|---|
| $Fe^{3+}$+32$H_2O$ | 129 | $Fe^{2+}$+32$H_2O$ | 105 | $Fe^{3+}$+64$H_2O$ | 264 | $Fe^{2+}$+64$H_2O$ | 69 |
| $Fe^{3+}$+96$H_2O$ | 105 | $Fe^{2+}$+96$H_2O$ | 46 | $Cu^{2+}$+32$H_2O$ | 202 | $Cu^{+}$+32$H_2O$ | 177 |
| $Cu^{2+}$+64$H_2O$ | 78 | $Cu^{+}$+64$H_2O$ | 191 | $Cu^{2+}$+96$H_2O$ | 51 | $Cu^{+}$+96$H_2O$ | 78 |
| $Ag^{2+}$+32$H_2O$ | 153 | $Ag^{+}$+32$H_2O$ | 220 | $Ag^{2+}$+64$H_2O$ | 164 | $Ag^{+}$+64$H_2O$ | 201 |
| $Ag^{2+}$+96$H_2O$ | 49 | $Ag^{+}$+96$H_2O$ | 63 | 128$H_2O$ slab | 222 | | |

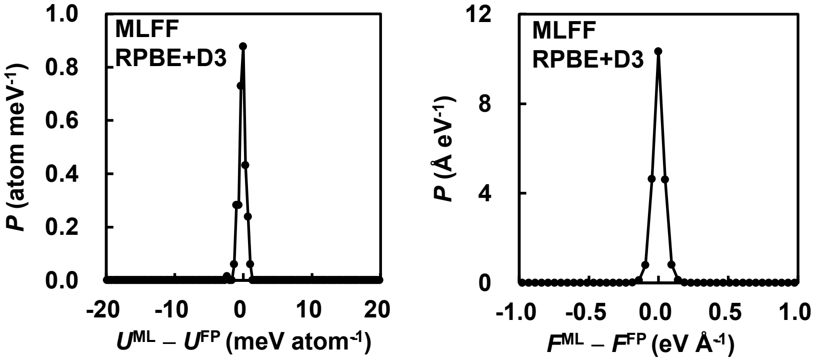


Figure S 1. Probability densities $P$ to find specific differences between the ML and FP results for the 128 $H_2O$ slab. $U$ and $F$ denote the potential energy and force, respectively. The superscript 'ML' and 'FP' indicate the values calculated by the MLFF model and the FP method using the semi-local RPBE+D3 functional ($FP_{sl}$ method).

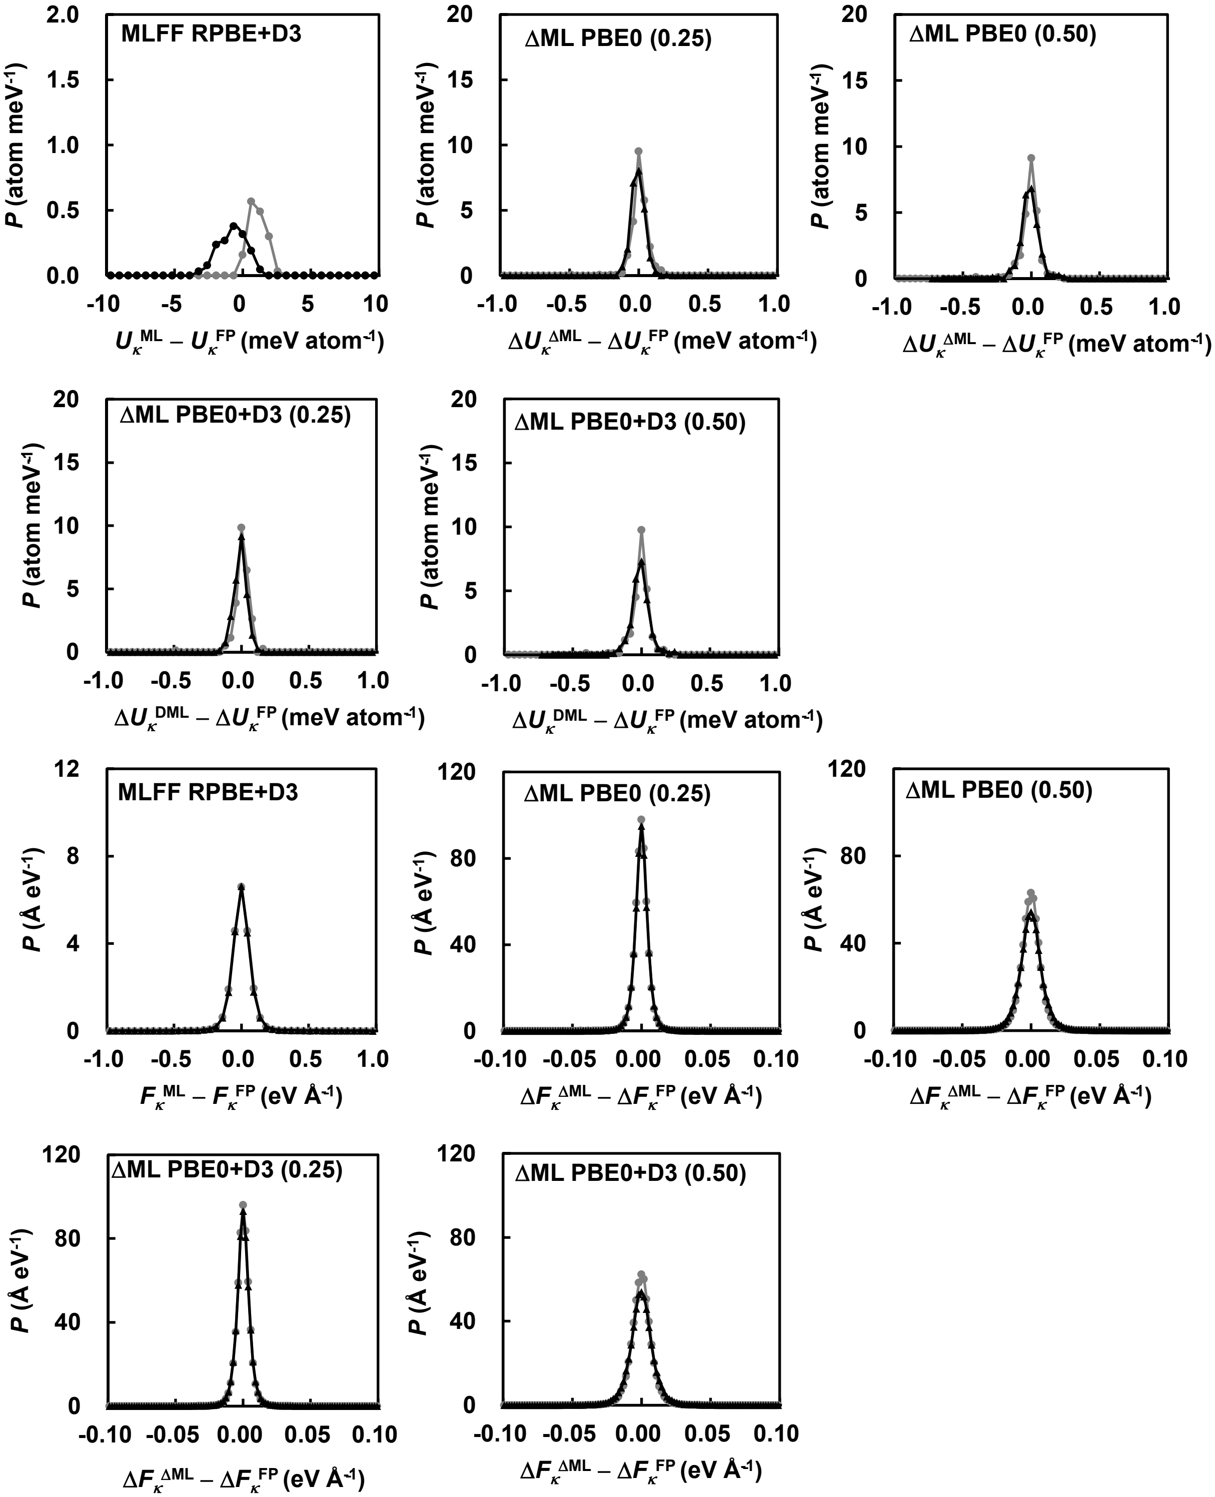


Figure S 2. Probability densities $P$ to find specific differences between the ML and FP results for the $Fe^{3+}$+64$H_2O$ (black) and $Fe^{2+}$+64$H_2O$ (gray) bulk solutions. $U_\kappa$ and $F_\kappa$ denote the potential energy and force, respectively, at the state $\kappa$ ($\kappa$=0 for the oxidized state and $\kappa = 1$ for the reduced state). $\Delta U_\kappa$ and $\Delta F_\kappa$ denote the differences of the potential energy and force, respectively, between the hybrid functional [(PBE0 (0.25), PBE0 (0.50), PBE0+D3 (0.25) and PBE0+D3 (0.50)] ($FP_{nl}$ method) and the semi-local functional (RPBE+D3) ($FP_{sl}$ method). The superscript 'ΔML' and 'FP' indicate the values calculated by the Δ-ML models and the FP method.

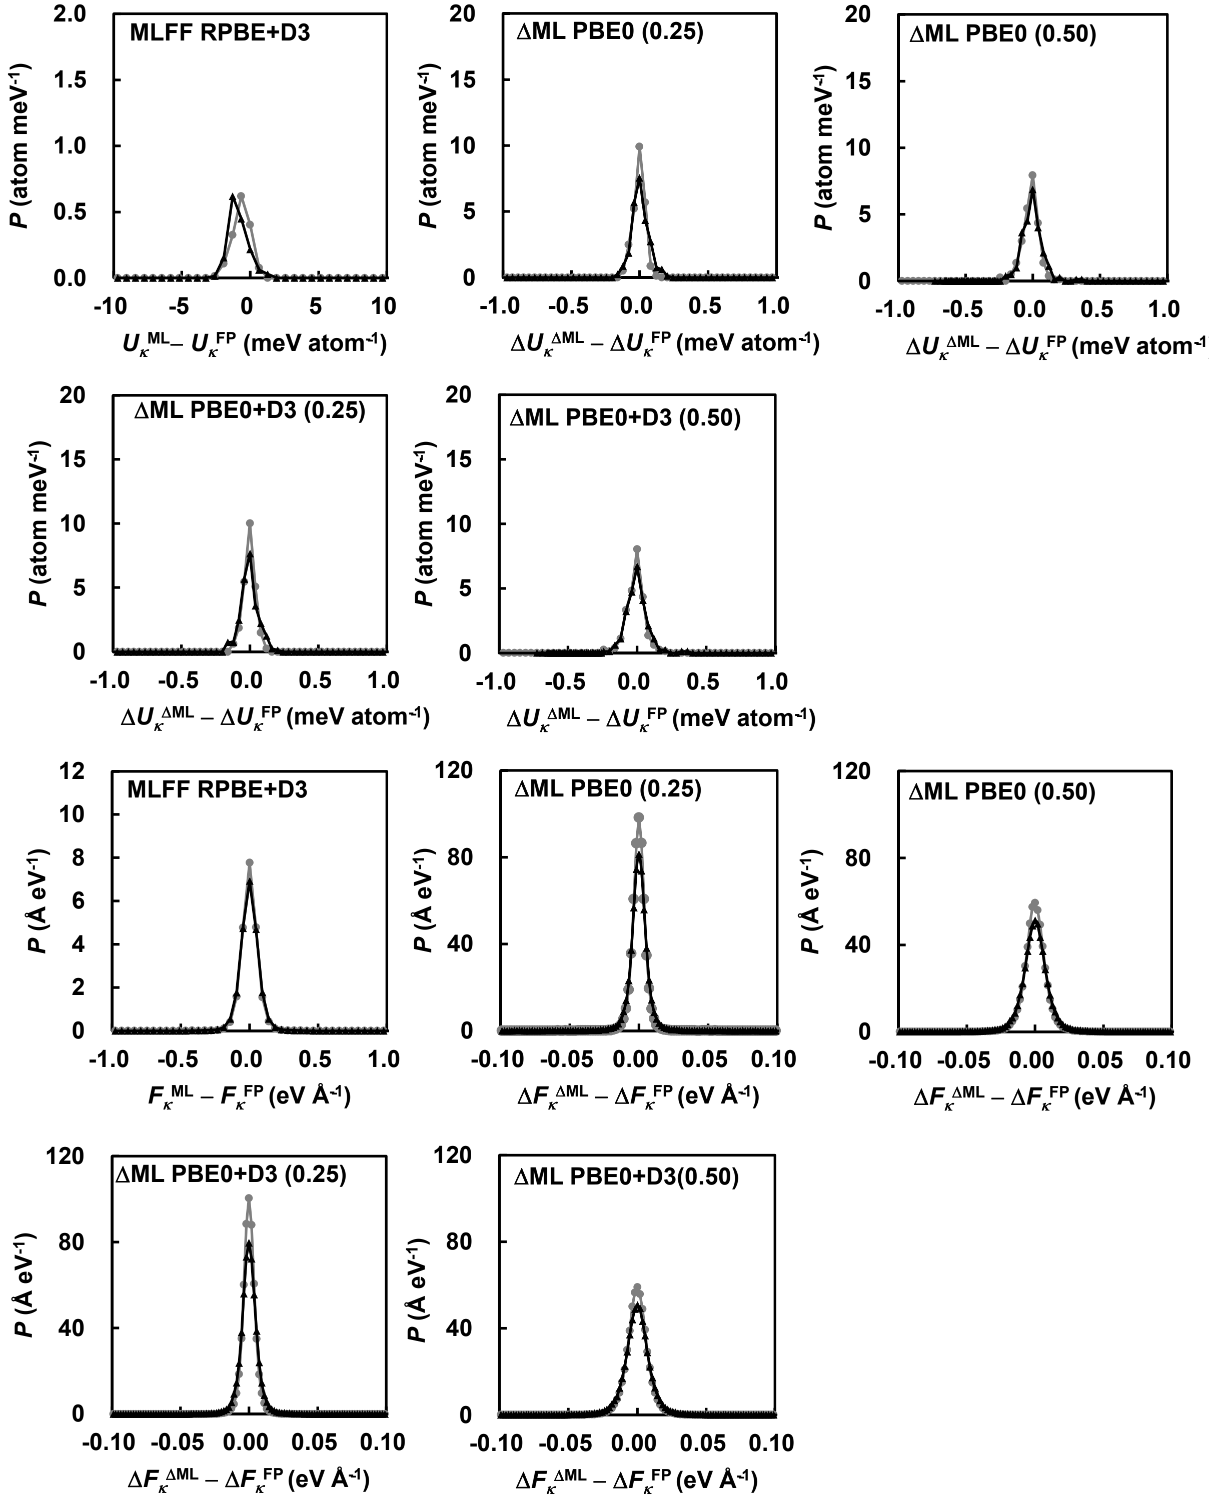


Figure S 3. Probability densities $P$ to find specific differences between the ML and FP results for the $Cu^{2+}$+64$H_2O$ (black) and $Cu^{+}$+64$H_2O$ (gray) bulk solutions. Notations are the same as those in Fig. S2.

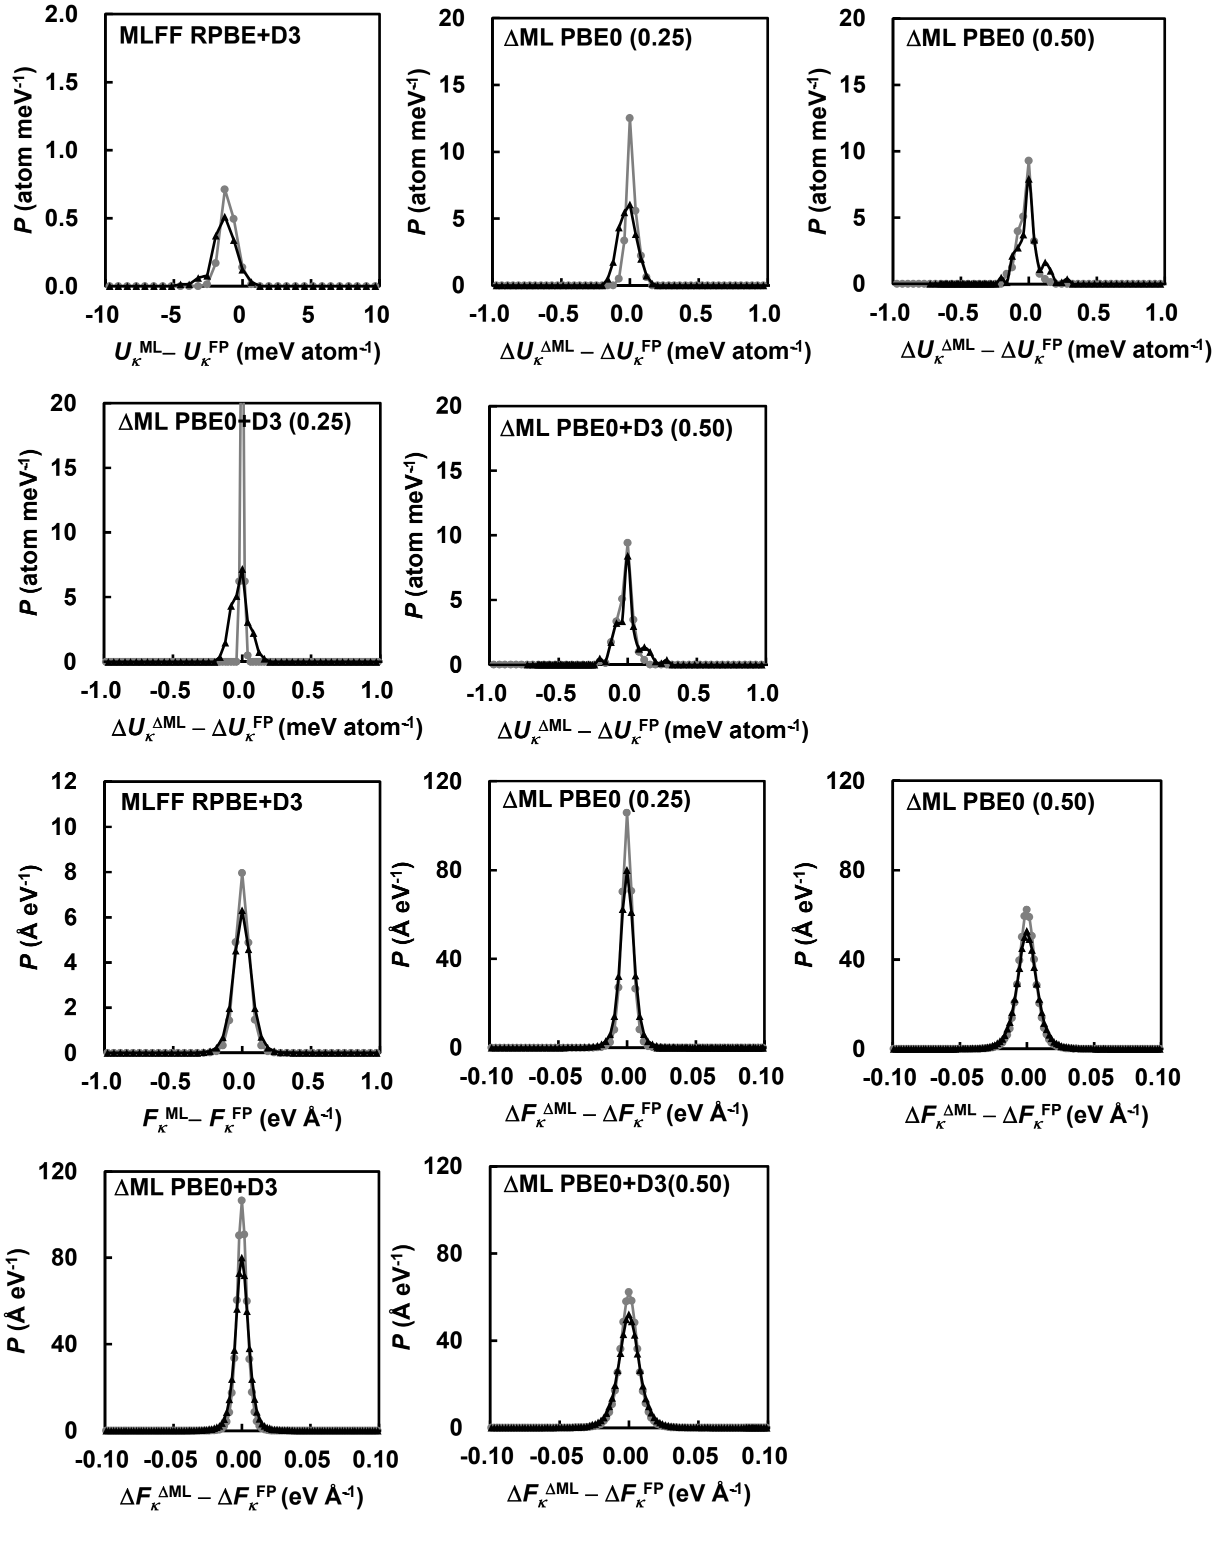


Figure S 4. Probability densities $P$ to find specific differences between the ML and FP results for the $Ag^{2+}$+64$H_2O$ (black) and $Ag^{+}$+64$H_2O$ (gray) bulk solutions. Notations are the same as those in Fig. S2.

## S2. ESTIMATION OF COMPUTE TIME

The compute times required for the brute-force method and our ML-aided method were estimated based on the measured elapsed time listed in Table S3. For both methods, bottleneck runs are in the calculations on the water slab and TI for the bulk solution systems. The estimation for each run is explained below.

*Calculation of oxygen 1s level in water slab:* For the brute-force method, a computationally expensive simulation is the total 1.5 ns MD simulation generating statistical independent configurations which are indispensable to obtain the flat local potential profile at the middle of the slab as shown in the inset of Fig. 1 in the main text. The compute time required for the FPMD simulation using the semi-local functional is approximately 1 mio core hours assuming the time step of 1 fs. In our ML-aided scheme, the bottleneck run is the FP calculations using the semi-local functional on 3000 structures selected randomly from the MD trajectories generated by the MLFF surrogate model and on 222 structures used for training because the compute time for the ML run is negligibly small as shown in Table S3. The required compute time is 2200 core hours.

*Thermodynamic integration:* For the brute-force method, the most expensive computation is the TI simulation with using the hybrid functional. The compute time is approximately 20 mio core hours based on the elapsed time for the PBE0 functional shown in Table S3. Here, we assume 5 grids along the coupling-path $\lambda$ and a 100-ps-FPMD simulation for each oxidized and reduced state at each grid similarly to our TI with using the MLFF models. In our scheme, the bottleneck is in the 70-ps-FPMD simulations using the semi-local functional for the oxidized and reduced states, which cost approximately 16800 core hours.

Table S 3. Elapsed time (s) per MD step for the MLFFs compared to FP calculations using RPBE+D3 and PBE0 (0.25). Here, we show the timing for the $64H_2O$ bulk system, the $128H_2O$ slab system, and the $1024H_2O$ slab system, as typical examples.The elapsed time was measured by using 16 cores of Intel Xeon Platinum 8358 (2.6 GHz) for the MLFFs and RPBE+D3 calculations. For the PBE0 (0.25) calculations, 32 cores of the same machine were used.

| Method | System | Time | System | Time | System | Time |
|---|---|---|---|---|---|---|
| MLFF | $64H_2O$ bulk | 0.11 | $128H_2O$ slab | 0.10 | $1024H_2O$ slab | 0.42 |
| RPBE+D3 | $64H_2O$ bulk | 27 | $128H_2O$ slab | 154 | | |
| PBE0(0.25) | $64H_2O$ bulk | 2313 | $128H_2O$ slab | 14974 | | |

## S3. SUPPLEMENTARY DATA FOR WATER SLABS

Orientational distributions of water dipole vectors and OH-bonds near the Gibbs dividing surfaces in the slabs of 128 and 1024 water molecules per unit cell are shown in Fig. S5. Here, the Gibbs dividing surface is defined as the surface, where the water density equals to a half of the bulk density. The distribution for the 128 molecular system was calculated from total of 37500 structures selected from 15 MD trajectories obtained by using the MLFF trained on the $FP_{sl}$ (RPBE+D3) data. Each trajectory was generated by a 100-ps-NVT-ensemble MD simulation at 298 K. The distribution for the 1024 molecular system was calculated from total of 7500 structures selected from 3 MD trajectories generated by 100-ps-NVT-ensemble MD simulations at 298 K.

Figure S6 shows the time evolution of the oxygen 1s level of water molecules at the middle of the slab comprising 128 water molecules, as well as the one of water molecules far from the redox species in the bulk solutions. In the same figure, the mean value of the core level is shown as a function of the number of data. Statistically accurate result can be obtained by 2000 structures for the slab and 300 structures for the bulk solutions.

Figure S7 shows the density and local potential profiles averaged over a total of 3000 structures of the 128 molecular system. Here, the local potential obtained by using the $FP_{sl}$ method is shown. The local potential averaged in the shaded region provides the well-converged value of $3.65 \pm 0.02$ V scaled to the middle of the vacuum. Similarly, 1s levels of oxygen atoms in the shaded region were averaged. In Table S4, the calculated value $\varepsilon_{1s,slab}$ is compared to the one $\varepsilon_{1s,bulk}$ for the bulk pristine water modelled by 64 water molecules per unit cell. In Table S5, the difference, $\Delta\bar{\phi} = \varepsilon_{1s,bulk} - \varepsilon_{1s,slab}$, for the pure water is tabulated (see lines of $64H_2O$). The difference $3.64 \pm 0.02$ V calculated by the $FP_{sl}$ method is consistent with the value calculated from the local potential within the error bars estimated by the block averaging analysis [1]. Because the $FP_{sl}$ method already gives the accurate electrostatic potential, the change in the oxygen 1s level and local potential with changing the XC functional to the non-local hybrid functional is small. The small deviation can be efficiently computed by averaging the differences over 30 configurations for each bulk and slab system. The results are also tabulated in Table S4 and Table S5.

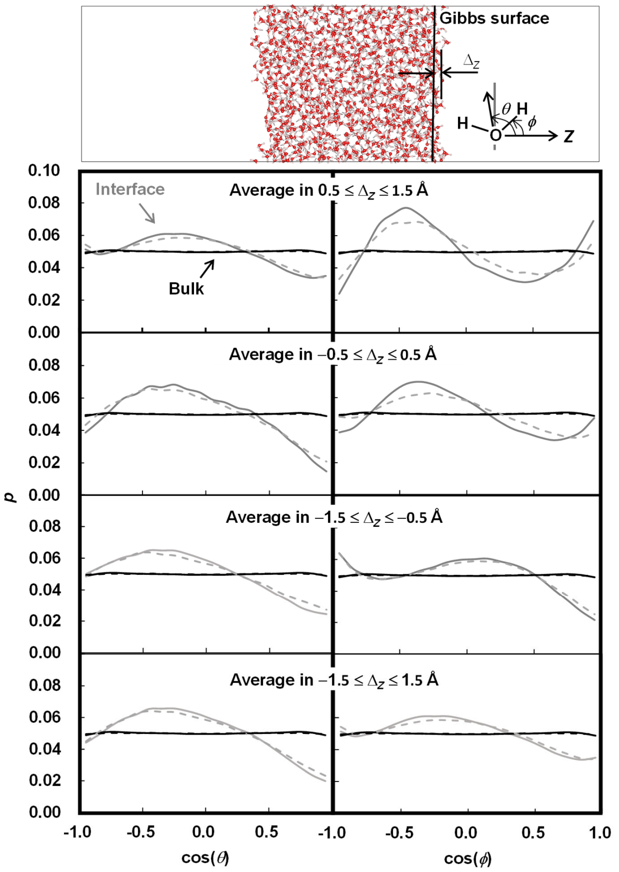


Figure S 5. Orientation distribution of water dipole vectors and OH-bonds relative to the surface normal direction $Z$. Solid and dashed lines are the results for the slabs composed of 128 and 1024 water molecules, respectively. Black and gray lines are the results for the bulk and interfacial regions, respectively. For the interface, orientations of water molecules in a 1 Å slice centered at $-1$, 0 and 1 Å from the Gibbs dividing surface are examined. Here, the symbol $\Delta_Z$ means the distance from the Gibbs dividing surface. The bulk region is defined as a 7 Å slice centered at the middle of the water slab.

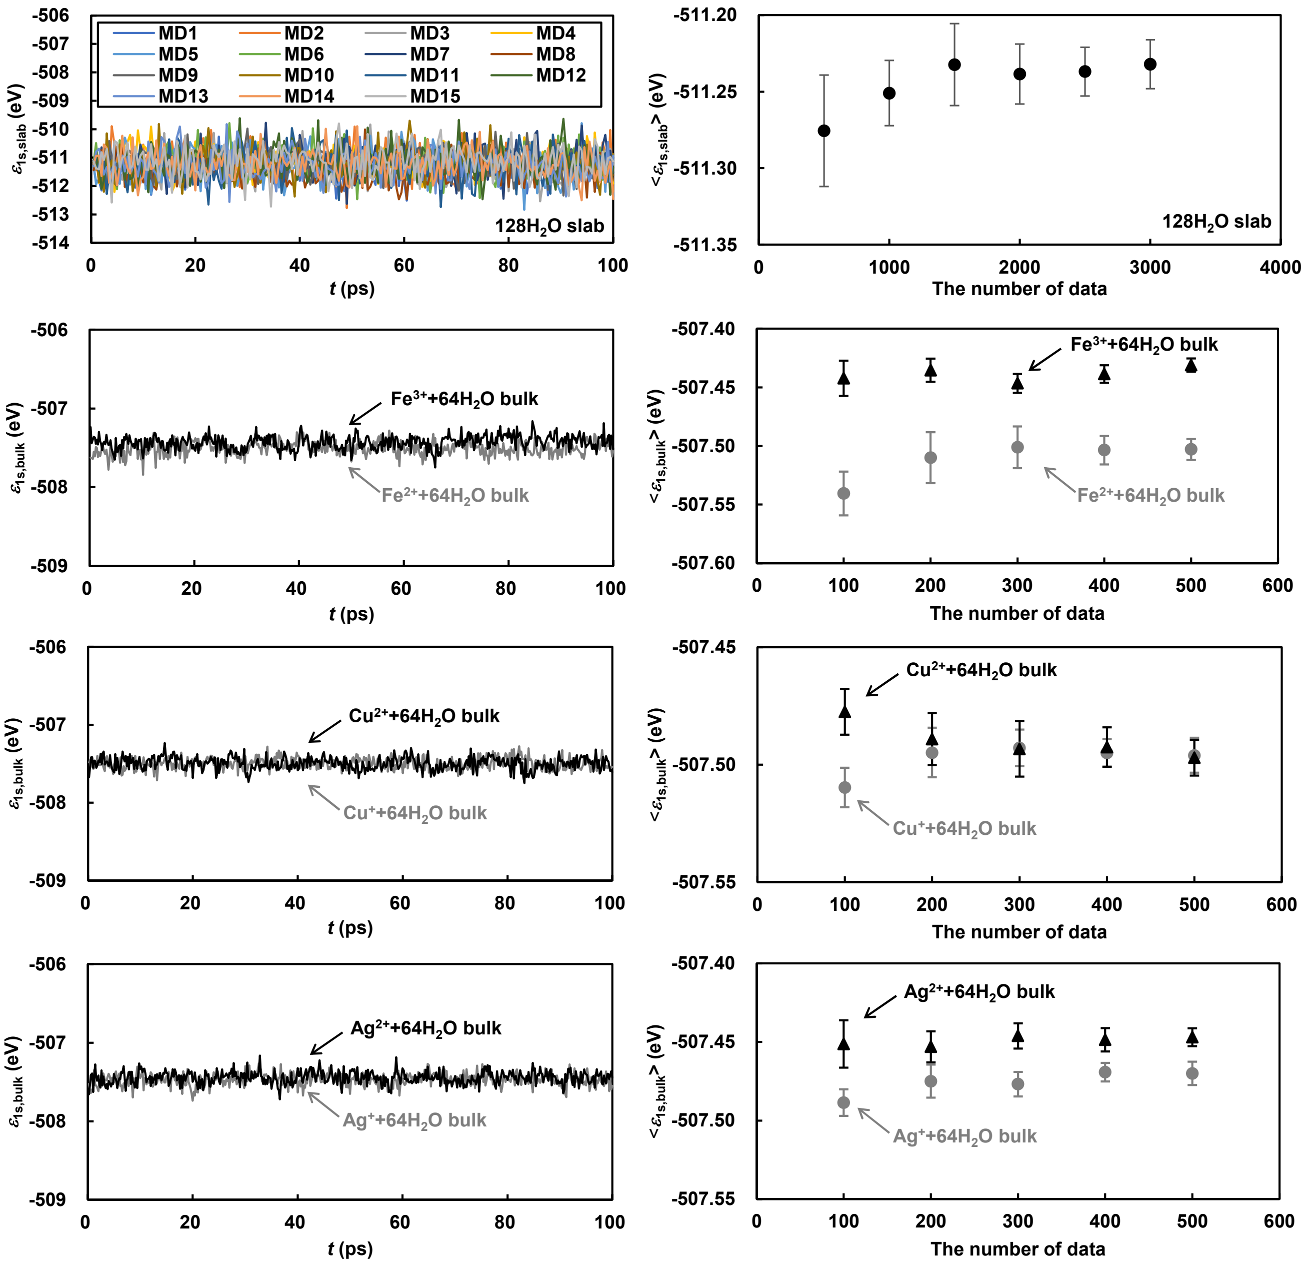


Figure S 6. Time evolution of the oxygen 1s level of water molecules at the middle of the slab comprising 128 water molecules ($\varepsilon_{1s,slab}$), as well as the one of water molecules far from the redox species in the bulk solutions ($\varepsilon_{1s,bulk}$). Their averages $\langle \varepsilon_{1s,slab} \rangle$ and $\langle \varepsilon_{1s,bulk} \rangle$ are also shown as functions of the number of data.

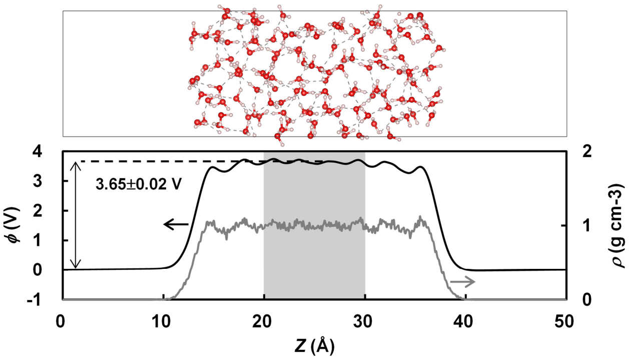


Figure S 7. Local potential $\phi$ and water density $\rho$ across the water slab comprised of 128 water molecules.

Table S 4. The averaged value of 1s levels of oxygen atoms in the bulk pristine water modelled by $64H_2O$, the one at the middle of the water slab modelled by $128H_2O$ slab ($\varepsilon_{1s,slab}$), and the one at the region far from the redox species in the bulk solutions ($\varepsilon_{1s,bulk}$). Here, $\varepsilon_{1s,slab}$ is scaled to the local potential at the middle of the vacuum layer, while $\varepsilon_{1s,bulk}$ is scaled to the average of the local potential in the bulk system. Unit is in eV.

| System | $FP_{sl}$ (RPBE+D3) | $FP_{nl}$ [PBE0 (+D3) (0.25)] | $FP_{nl}$ [PBE0 (+D3) (0.50)] |
|---|---|---|---|
| $128H_2O$ slab | −511.23±0.02 | −511.12±0.02 | −511.05±0.02 |
| $64H_2O$ | −507.59±0.01 | −507.60±0.01 | −507.62±0.01 |
| $Fe^{3+}$+$32H_2O$ ($\lambda$=0) | −507.42±0.01 | | |
| $Fe^{2+}$+$32H_2O$ ($\lambda$=1) | −507.48±0.01 | | |
| $Fe^{3+}$+$64H_2O$ ($\lambda$=0) | −507.43±0.01 | −507.43±0.01 | −507.44±0.01 |
| $Fe^{2+}$+$64H_2O$ ($\lambda$=1) | −507.50±0.01 | −507.52±0.01 | −507.54±0.01 |
| $Fe^{3+}$+$96H_2O$ ($\lambda$=0) | −507.43±0.01 | | |
| $Fe^{2+}$+$96H_2O$ ($\lambda$=1) | −507.52±0.01 | | |
| $Cu^{2+}$+$32H_2O$ ($\lambda$=0) | −507.47±0.01 | | |
| $Cu^{+}$+$32H_2O$ ($\lambda$=1) | −507.43±0.01 | | |
| $Cu^{2+}$+$64H_2O$ ($\lambda$=0) | −507.50±0.01 | −507.51±0.01 | −507.50±0.01 |
| $Cu^{+}$+$64H_2O$ ($\lambda$=1) | −507.47±0.01 | −507.52±0.01 | −507.53±0.01 |
| $Cu^{2+}$+$96H_2O$ ($\lambda$=0) | −507.50±0.01 | | |
| $Cu^{+}$+$96H_2O$ ($\lambda$=1) | −507.51±0.01 | | |
| $Ag^{2+}$+$32H_2O$ ($\lambda$=0) | −507.31±0.01 | | |
| $Ag^{+}$+$32H_2O$ ($\lambda$=1) | −507.36±0.01 | | |
| $Ag^{2+}$+$64H_2O$ ($\lambda$=0) | −507.45±0.01 | −507.43±0.01 | −507.44±0.01 |
| $Ag^{+}$+$64H_2O$ ($\lambda$=1) | −507.47±0.01 | −507.48±0.01 | −507.51±0.01 |
| $Ag^{2+}$+$96H_2O$ ($\lambda$=0) | −507.47±0.01 | | |
| $Ag^{+}$+$96H_2O$ ($\lambda$=1) | −507.49±0.01 | | |

Table S 5. The difference $e\Delta\bar{\phi}$ between the oxygen 1s level at the middle of the 128 water slab scaled to the vacuum and the one at the region far away from the metal cations in the bulk solution scaled to the average of the local potential in the same unit cell. $\Delta\bar{\phi}$ are calculated from the data tabulated Table S4. The difference between the oxygen 1s level for slab and the one for the bulk pristin water is also shown. Unit of $\Delta\bar{\phi}$ is V.

| System | XC functional | $\Delta\bar{\phi}$ |
|---|---|---|
| $64H_2O$ | $FP_{sl}$ (RPBE+D3) | 3.64±0.02 |
| $64H_2O$ | $FP_{nl}$ [PBE0 (0.25)] | 3.52±0.02 |
| $64H_2O$ | $FP_{nl}$ [PBE0+D3 (0.25)] | 3.52±0.02 |
| $64H_2O$ | $FP_{nl}$ [PBE0 (0.50)] | 3.44±0.02 |
| $64H_2O$ | $FP_{nl}$ [PBE0+D3 (0.50)] | 3.44±0.02 |
| $Fe^{3+}/Fe^{2+}+32H_2O$ | $FP_{sl}$ (RPBE+D3) | 3.79±0.02 |
| $Fe^{3+}/Fe^{2+}+64H_2O$ | $FP_{sl}$ (RPBE+D3) | 3.77±0.02 |
| $Fe^{3+}/Fe^{2+}+64H_2O$ | $FP_{nl}$ [PBE0 (0.25)] | 3.65±0.02 |
| $Fe^{3+}/Fe^{2+}+64H_2O$ | $FP_{nl}$ [PBE0+D3 (0.25)] | 3.65±0.02 |
| $Fe^{3+}/Fe^{2+}+64H_2O$ | $FP_{nl}$ [PBE0 (0.50)] | 3.56±0.02 |
| $Fe^{3+}/Fe^{2+}+64H_2O$ | $FP_{nl}$ [PBE0+D3 (0.50)] | 3.56±0.02 |
| $Fe^{2+}/Fe^{2+}+96H_2O$ | $FP_{sl}$ (RPBE+D3) | 3.76±0.02 |
| $Cu^{2+}/Cu^{+}+32H_2O$ | $FP_{sl}$ (RPBE+D3) | 3.79±0.02 |
| $Cu^{2+}/Cu^{+}+64H_2O$ | $FP_{sl}$ (RPBE+D3) | 3.74±0.02 |
| $Cu^{2+}/Cu^{+}+64H_2O$ | $FP_{nl}$ [PBE0 (0.25)] | 3.61±0.02 |
| $Cu^{2+}/Cu^{+}+64H_2O$ | $FP_{nl}$ [PBE0+D3 (0.25)] | 3.61±0.02 |
| $Cu^{2+}/Cu^{+}+64H_2O$ | $FP_{nl}$ [PBE0 (0.50)] | 3.54±0.02 |
| $Cu^{2+}/Cu^{+}+64H_2O$ | $FP_{nl}$ [PBE0+D3 (0.50)] | 3.54±0.02 |
| $Cu^{2+}/Cu^{+}+96H_2O$ | $FP_{sl}$ (RPBE+D3) | 3.73±0.03 |
| $Ag^{2+}/Ag^{+}+32H_2O$ | $FP_{sl}$ (RPBE+D3) | 3.90±0.02 |
| $Ag^{2+}/Ag^{+}+64H_2O$ | $FP_{sl}$ (RPBE+D3) | 3.78±0.02 |
| $Ag^{2+}/Ag^{+}+64H_2O$ | $FP_{nl}$ [PBE0 (0.25)] | 3.67±0.02 |
| $Ag^{2+}/Ag^{+}+64H_2O$ | $FP_{nl}$ [PBE0+D3 (0.25)] | 3.67±0.02 |
| $Ag^{2+}/Ag^{+}+64H_2O$ | $FP_{nl}$ [PBE0 (0.50)] | 3.58±0.02 |
| $Ag^{2+}/Ag^{+}+64H_2O$ | $FP_{nl}$ [PBE0+D3 (0.50)] | 3.58±0.02 |
| $Ag^{2+}/Ag^{+}+96H_2O$ | $FP_{sl}$ (RPBE+D3) | 3.76±0.02 |

## S4. SUPPLEMENTARY FIGURES FOR TI AND TPT

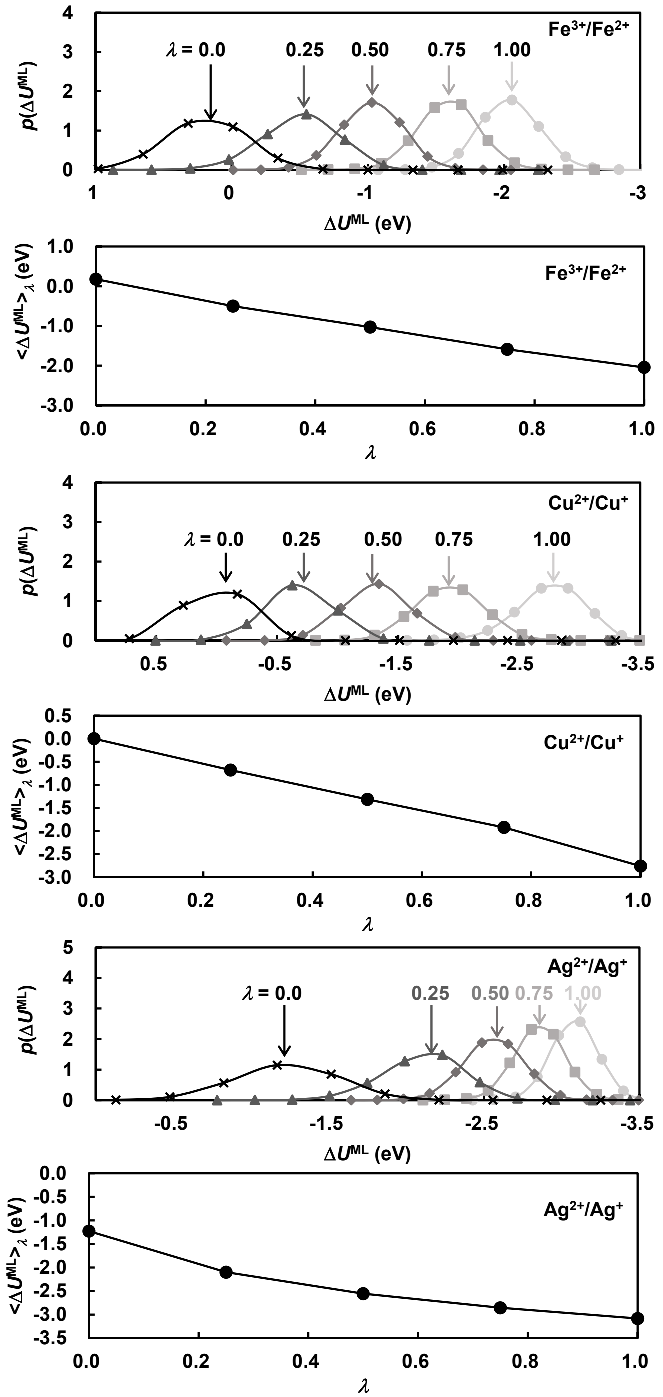


Figure S 8. Probability distributions of $\partial H^{\mathrm{ML}}/\partial\lambda = \Delta U^{\mathrm{ML}}$ in the MD simulations for the TI calculations employing the MLFFs and their averages for $Fe^{3+}$/$Fe^{2+}$, $Cu^{2+}$/$Cu^{+}$ and $Ag^{2+}$/$Ag^{+}$ redox couples as functions of the coupling parameter $\lambda$.

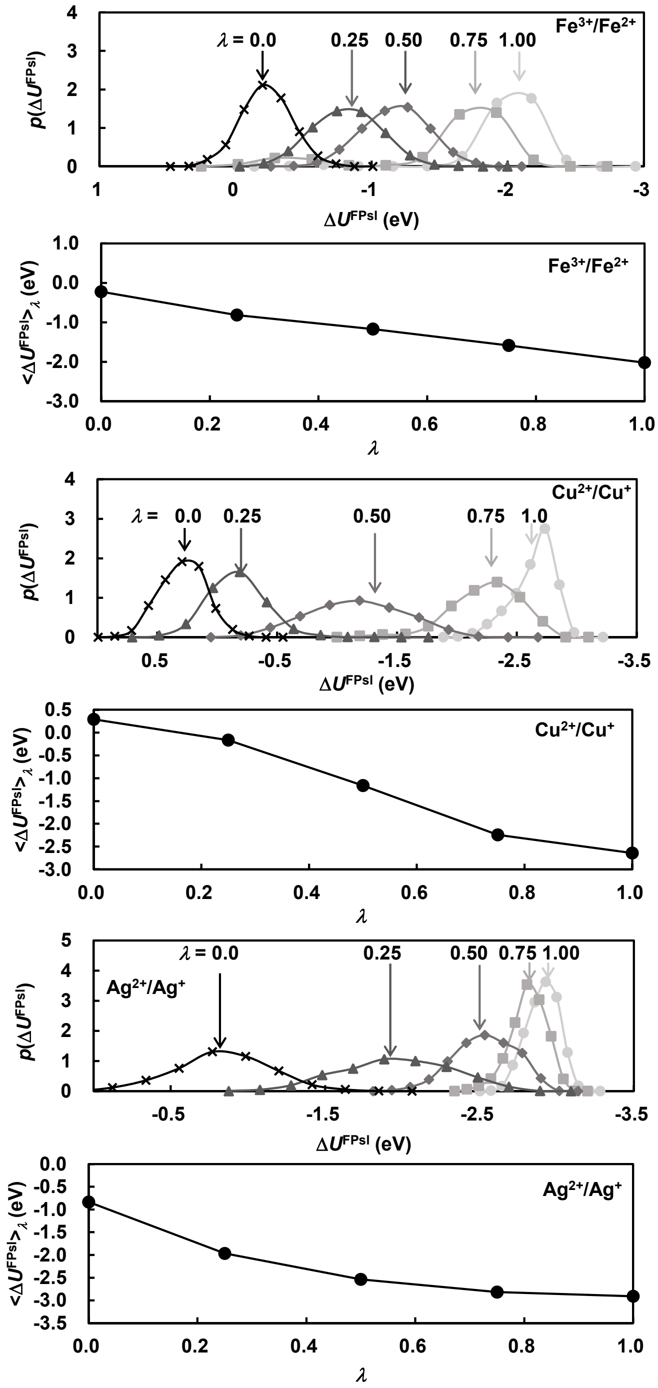


Figure S 9. Probability distributions of $\partial H^{\mathrm{FP_{sl}}}/\partial\lambda = \Delta U^{\mathrm{FP_{sl}}}$ in the MD simulations for the TI calculations employing the semi-local functional (RPBE+D3) and their averages for $Fe^{3+}$/$Fe^{2+}$, $Cu^{2+}$/$Cu^{+}$ and $Ag^{2+}$/$Ag^{+}$ redox couples as functions of the coupling parameter $\lambda$.

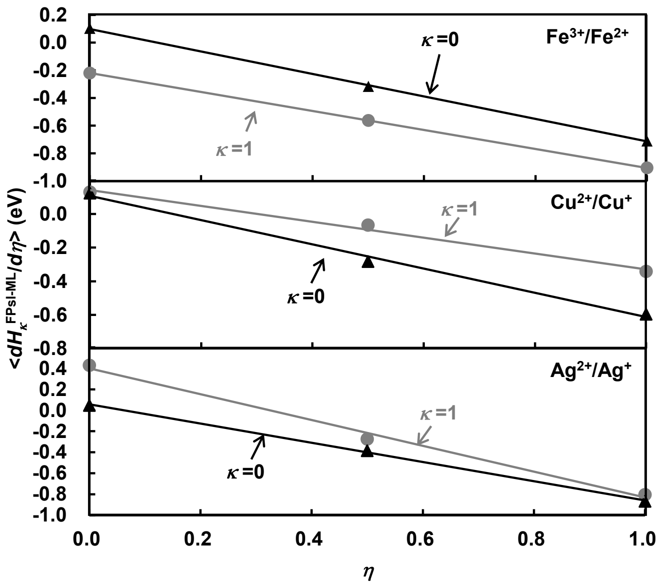


Figure S 10. Integrand $< dH_{\kappa}^{\mathrm{FP_{sl}-ML}}/d\eta >_{\eta}$ of Eqs. (13) and (14) in the main text.

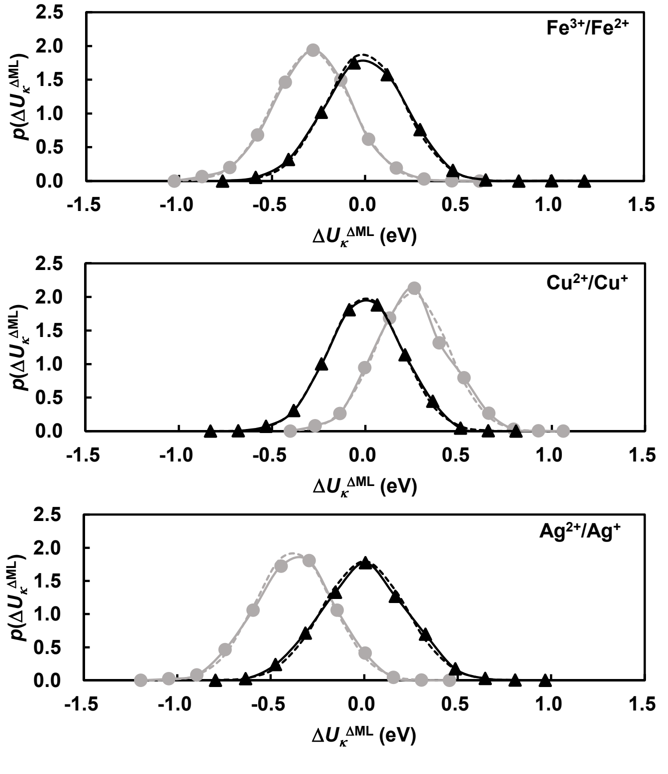


Figure S 11. Probability distributions of energy difference $\Delta U_{\kappa}^{\Delta\mathrm{ML}}$ for the PBE0+D3 ($x$=0.25) functional. Black and gray lines and symbols are the distributions for the oxidized ($\kappa$=0) and reduced ($\kappa$=1) states, respectively. Dashed lines show Gaussian distributions fitted to the raw data. Here, energy difference is shifted so that the center of energy difference for the oxidized state becomes zero. Distributions for other functionals (not shown in the figure) are also described well by Gaussian distributions.

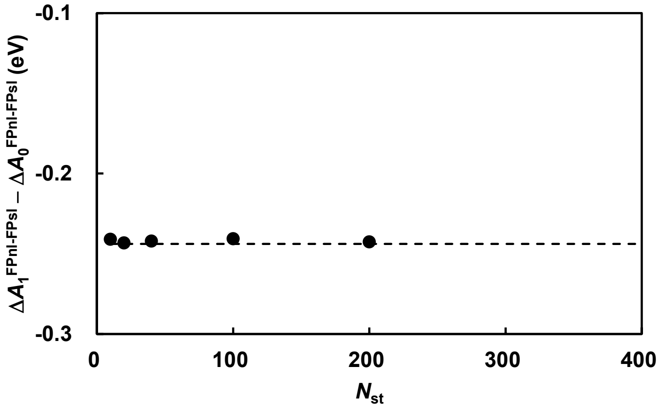


Figure S 12. Free energy difference $\Delta A_1^{\mathrm{FP_{nl}-FP_{sl}}} - \Delta A_0^{\mathrm{FP_{nl}-FP_{sl}}}$ for the $Fe^{3+}/Fe^{2+}$ couple calculated by using Δ-ML models trained on differences of energies and forces of $N_{\mathrm{st}}$ structures. Here, the ensemble average in Eq. (15) is taken over 400 structures. The dashed line shows the value of the difference calculated by using FP potential energy differences between the $\mathrm{FP_{nl}}$ [PBE0 (0.25)] and $\mathrm{FP_{sl}}$ (RPBE+D3) methods for all 400 structures instead of $\Delta U_\kappa^{\Delta \mathrm{ML}}$.

## S5. SUPPLEMENTARY DATA FOR REDOX POTENTIALS

Table S6 summarizes the redox potentials $U_{redox}$ calculated by the method relevant to the $FP_{sl}$ (RPBE+D3) method. The lines of ML show the values calculated using the MLFFs trained on $FP_{sl}$. Here, the values were calculated from $\Delta A^{ML}$ in Eq. (11) without any correction. The lines of $FP_{sl}$ w/ ML show the values obtained by correcting $\Delta A^{ML}$ via Eq. (13). The values in the lines of $FP_{sl}$ w/o ML are the results obtained from Eqs. (18) and (19) without using the MLFFs.

Figure S13 shows $U_{redox}$ of $FP_{sl}$ ($FP_{sl}$ w/ ML) as a function of the number of water molecules in the unit cell of the bulk solution systems.

Table S7 shows $U_{redox}$ calculated by five XC functionals with the statistical error bars ($2\sigma$) of the mean values. Here, the standard deviation $\sigma$ was determined by propagating errors of $\Delta\bar{\phi}$ and all relevant quantities in Eqs. (16) and (17) using the block averaging analysis [1].

All redox potentials shown in the tables and figure were calculated using $\Delta\bar{\phi}$ defined as Eq. (8) in the main text and tabulated in Table S 5. The oxygen 1s level at the middle of the water slab ($\varepsilon_{1s,slab}$) was calculated by the method explained in Section S3. The one in the bulk solution ($\varepsilon_{1s,bulk}$) was calculated by averaging over all oxygen atoms $L/2$ away from the metal cations, where $L$ means the length of the side of the unit cell.The oxygen 1s levels for the slab and the bulk solutions were tabulated in Table S4.

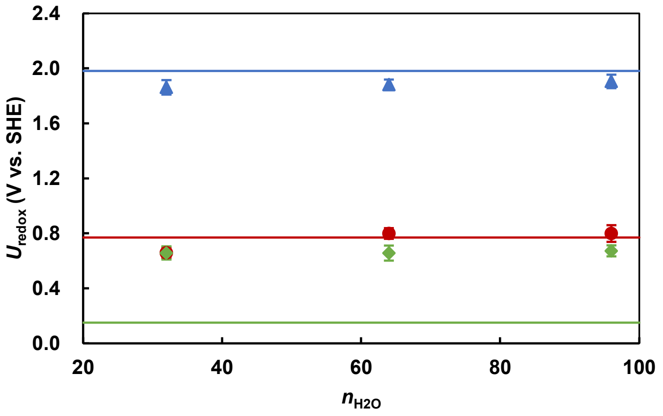


Figure S 13. Redox potentials calculated by the $FP_{sl}$ method (RPBE+D3) as functions of the number of water molecules $n_{H_2O}$ per unit cell. Red circles, green diamonds, and blue triangles are the calculated redox potentials of $Fe^{3+}/Fe^{2+}$, $Cu^{2+}/Cu^{+}$ and $Ag^{2+}/Ag^{+}$ couples, respectively. Solid lines show the experimental redox potentials.

Table S 6. The redox potentials ($U_{\text{redox}} = -\Delta A/e$) [V in vacuum scale (values in parenthesis are in SHE scale)] calculated by three methods relevant to the $FP_{sl}$ (RPBE+D3) (see text in SI for their details). The local potential differences $\Delta\bar{\phi}$ tabulated in Table S5 are used. The absolute potential of SHE is set to 4.44 V [2]. Experimental redox potentials are taken from Ref. [3].

| System | Method | $U_{\text{redox}}$ |
|---|---|---|
| $Fe^{3+}/Fe^{2+}+32H_2O$ | ML | 4.86 (0.42)±0.02 |
| | $FP_{sl}$ w/ ML | 5.10 (0.66)±0.04 |
| | $FP_{sl}$ w/o ML | 5.13 (0.69)±0.03 |
| $Fe^{3+}/Fe^{2+}+64H_2O$ | ML | 4.99 (0.55)±0.03 |
| | $FP_{sl}$ w/ ML | 5.24 (0.80)±0.04 |
| | $FP_{sl}$ w/o ML | 5.17 (0.73)±0.06 |
| $Fe^{3+}/Fe^{2+}+96H_2O$ | ML | 5.41 (0.97)±0.02 |
| | $FP_{sl}$ w/ ML | 5.24 (0.80)±0.06 |
| | $FP_{sl}$ w/o ML | 5.26 (0.82)±0.04 |
| $Fe^{3+}/Fe^{2+}$ | Exp. | 5.21 (0.77) |
| $Cu^{2+}/Cu^{+}+32H_2O$ | ML | 5.12 (0.68)±0.04 |
| | $FP_{sl}$ w/ ML | 5.10 (0.66)±0.05 |
| | $FP_{sl}$ w/o ML | 5.04 (0.60)±0.04 |
| $Cu^{2+}/Cu^{+}+64H_2O$ | ML | 5.27 (0.83)±0.04 |
| | $FP_{sl}$ w/ ML | 5.10 (0.66)±0.05 |
| | $FP_{sl}$ w/o ML | 5.13 (0.69)±0.07 |
| $Cu^{2+}/Cu^{+}+96H_2O$ | ML | 5.17 (0.73)±0.03 |
| | $FP_{sl}$ w/ ML | 5.11 (0.67)±0.04 |
| | $FP_{sl}$ w/o ML | 5.17 (0.73)±0.06 |
| $Cu^{2+}/Cu^{+}$ | Exp. | 4.59 (0.15) |
| $Ag^{2+}/Ag^{+}+32H_2O$ | ML | 6.42 (1.98)±0.04 |
| | $FP_{sl}$ w/ ML | 6.30 (1.86)±0.05 |
| | $FP_{sl}$ w/o ML | 6.27 (1.83)±0.06 |
| $Ag^{2+}/Ag^{+}+64H_2O$ | ML | 6.41 (1.97)±0.03 |
| | $FP_{sl}$ w/ ML | 6.32 (1.88)±0.04 |
| | $FP_{sl}$ w/o ML | 6.28 (1.84)±0.06 |
| $Ag^{2+}/Ag^{+}+96H_2O$ | ML | 6.44 (2.00)±0.03 |
| | $FP_{sl}$ w/ ML | 6.34 (1.90)±0.05 |
| | $FP_{sl}$ w/o ML | 6.28 (1.84)±0.05 |
| $Ag^{2+}/Ag^{+}$ | Exp. | 6.42 (1.98) |

Table S 7. Redox potentials $U_{\mathrm{redox}}$ of three redox couples calculated by RPBE+D3, PBE0 (0.25), PBE0 (0.50), PBE0+D3 (0.25) and PBE0+D3 (0.50) with the aid of the MLFF and Δ-ML. Their RMSEs compared to the experimental redox potentials are also shown. Here, the results for 64 water molecular systems are shown. The absolute potential of SHE is set to 4.44 V [2]. Experimental redox potentials are taken from Ref. [3].

| XC functional | $Fe^{3+}/Fe^{2+}$ | $Cu^{2+}/Cu^{+}$ | $Ag^{2+}/Ag^{+}$ | RMSE |
|---|---|---|---|---|
| RPBE+D3 | 0.80±0.04 | 0.66±0.05 | 1.88±0.04 | 0.29 |
| PBE0 ($x$=0.25) | 0.92±0.13 | 0.26±0.07 | 1.99±0.16 | 0.11 |
| PBE0 ($x$=0.50) | 0.79±0.15 | −0.34±0.18 | 2.12±0.16 | 0.30 |
| PBE0+D3 ($x$=0.25) | 0.94±0.13 | 0.24±0.07 | 2.02±0.10 | 0.11 |
| PBE0+D3 ($x$=0.50) | 0.83±0.15 | −0.38±0.19 | 2.13±0.14 | 0.32 |
| Exp. | 0.77 | 0.15 | 1.98 | |

## S6. SUPPLEMENTARY INFORMATION FOR VALIDATION OF TPT CALCULATION

The free energy difference ($\Delta A_{\kappa}^{\mathrm{FP_{nl}-FP_{sl}}}$) between the hybrid functional ($\mathrm{FP_{nl}}$) and semi-local functional ($\mathrm{FP_{sl}}$) was calculated using the TPT with second-order cumulant expansion, as described by Eq. (15) in the main text. However, the free energy difference might not converge if the two functionals lead to distinct differences in the solution structure. Therefore, we performed a verification of the TPT calculations in advance of the production runs. For this verification, we conducted TI and TPT simulations using MLFFs trained on the $\mathrm{FP_{nl}}$ and $\mathrm{FP_{sl}}$ data, denoted as $\mathrm{ML_{nl}}$ and $\mathrm{ML_{sl}}$, respectively. The $\mathrm{ML_{sl}}$ used here is the same as the one employed for the TI simulation explained in Methods section in the main text. $\mathrm{ML_{nl}}$ was trained on the energies, forces, and stress tensor components obtained by adding those predicted by the Δ-ML model to the $\mathrm{FP_{sl}}$ training data. The reference structures used for generating $\mathrm{ML_{sl}}$ were used for generating $\mathrm{ML_{nl}}$. Using $\mathrm{ML_{nl}}$ and $\mathrm{ML_{sl}}$ in the TI simulations, we calculated the free energy difference as:

$$\Delta A_{\kappa}^{\mathrm{ML_{nl}-ML_{sl}}} = \int_0^1 \left\langle \frac{\partial H_{\kappa}^{\mathrm{ML_{nl}-ML_{sl}}}}{\partial \eta} \right\rangle_{\eta} d\eta, \tag{S1}$$

$$H_{\kappa}^{\mathrm{ML_{nl}-ML_{sl}}} = \sum_{i=1}^{N_{\mathrm{a}}} \frac{|\mathbf{p}_i|^2}{2m_i} + \eta U_{\kappa}^{\mathrm{ML_{nl}}} + (1-\eta)\, U_{\kappa}^{\mathrm{ML_{sl}}}, \tag{S2}$$

where $U_{\kappa}^{\mathrm{ML_{nl}}}$ and $U_{\kappa}^{\mathrm{ML_{sl}}}$ are the potential energies of $\mathrm{ML_{nl}}$ and $\mathrm{ML_{sl}}$, respectively. The free energy difference was also approximately computed by the TPT with the second-order cumulant expansion as:

$$\begin{aligned}\Delta A_{\kappa}^{\mathrm{ML_{nl}-ML_{sl}}} \simeq & \left\langle \Delta U_{\kappa}^{\mathrm{ML}} \right\rangle_{\mathrm{ML_{sl}}} \\ & - \frac{\beta}{2} \left\langle \left( \Delta U_{\kappa}^{\mathrm{ML}} - \left\langle \Delta U_{\kappa}^{\mathrm{ML}} \right\rangle_{\mathrm{ML_{sl}}} \right)^2 \right\rangle_{\mathrm{ML_{sl}}},\end{aligned} \tag{S3}$$

where $\Delta U_{\kappa}^{\mathrm{ML}}$ is $U_{\kappa}^{\mathrm{ML_{nl}}} - U_{\kappa}^{\mathrm{ML_{sl}}}$. The accuracy of the approximate TPT calculation can be verified by comparing the free energy differences obtained by Eqs. (S1) and (S3). Errors of $\mathrm{ML_{nl}}$ are nearly identical to those in $\mathrm{ML_{sl}}$, indicating that TI and TPT simulations using $\mathrm{ML_{nl}}$ cannot yield sufficiently accurate $\mathrm{FP_{nl}}$ free energies without corrections that require expensive $\mathrm{FP_{nl}}$ computations for thousands of structures. Therefore, in this study, we opted for TPT simulations employing the Δ-ML models based on trajectories of the $\mathrm{FP_{sl}}$ method instead of the TI simulations using $\mathrm{ML_{nl}}$. While $\mathrm{ML_{nl}}$ does not provide free energies with satisfactory precision, this model can effectively

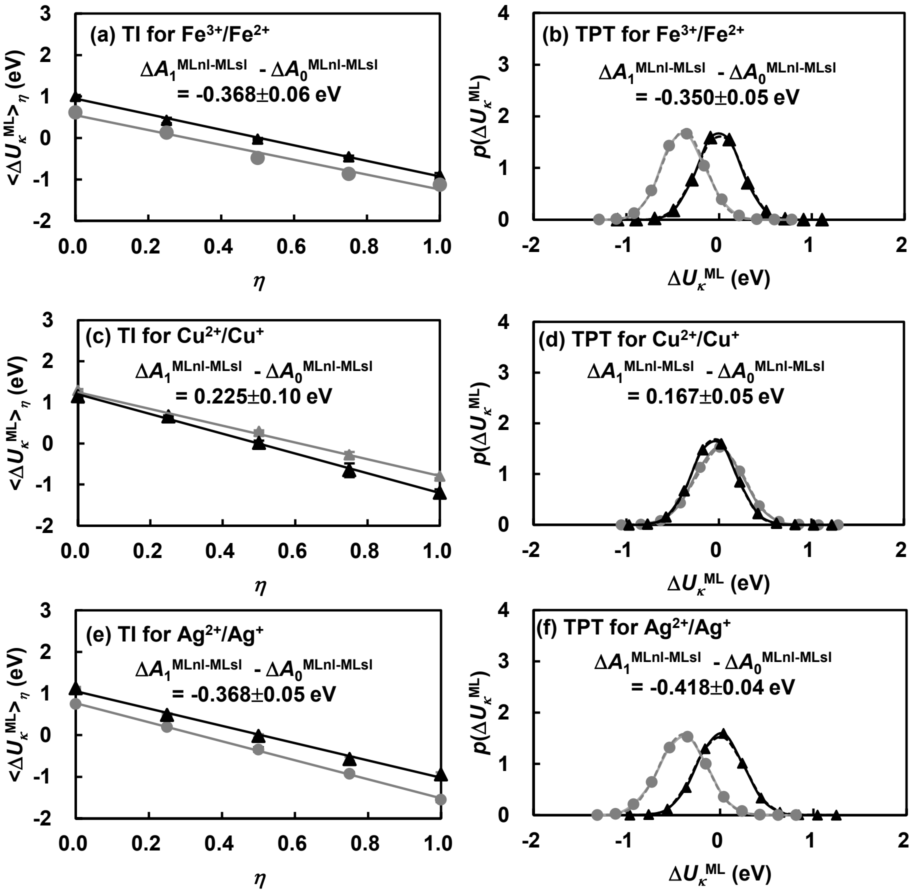


Figure S 14. Integrand of the TI Eq. (S1) [(a), (c) and (e)] and distribution of the energy difference $\Delta U_{\kappa}^{\mathrm{ML}} = U_{\kappa}^{\mathrm{ML_{nl}}} - U_{\kappa}^{\mathrm{ML_{sl}}}$ in Eq. (S3) [(b), (d) and (f)]. Black and gray lines and symbols show the results for the oxidized ($\kappa = 0$) and reduced states ($\kappa = 1$), respectively. Dashed lines show Gaussian distributions fitted to the raw data. Inset shows the calculated free energy difference $\Delta A_1^{\mathrm{ML_{nl}-ML_{sl}}} - \Delta A_0^{\mathrm{ML_{nl}-ML_{sl}}}$.

serve to verify the accuracy of TPT calculations.

The TI simulations were conducted using the Simpson's rule with five equidistant points. A 100-ps-NVT-ensemble MD simulation was performed for each grid point. The data for the TPT simulations were also obtained from these trajectories. The PBE0 hybrid functional and RPBE+D3 semi-local functional were used to train the MLFFs.

The simulated results are summarized in Fig. S14. The integrands of the TI simulations are roughly proportional to the coupling parameter $\eta$, and the distributions of $\Delta U_{\kappa}^{\mathrm{ML}}$ are reasonably represented by Gaussian distributions. Consequently, the TPT simulations reproduce the TI results within the statistical error range.

## S7. EFFECTS OF SEMI-CORE ELECTRON RELAXATIONS IN COPPER

To explain the specific free energy computations expalned in this subsection, we introduce additional abbreviations. Following the notations of PAWs in the VASP code, the PAWs with the electronic configurations, $3d^{10}4p^1$ and $3p^6 3d^{10}4p^1$, are denoted as 'sv' and 'pv', respectively. The $FP_{sl}$ methods using sv and pv are denoted as $FP_{sl}^{sv}$ and $FP_{sl}^{pv}$, respectively, and the $FP_{nl}$ method using pv is denoted as $FP_{nl}^{pv}$. The free energy computation using the $FP_{sl}^{sv}$ method is explained in the main text. Here, we explain the additional computation using pv, which was performed to examine the impact of semi-core electron relaxations.

The redox potential of the semi-local functional was computed by two types of TI simulations. One is a TI simulation from the potential calculated by the MLFF trained on the $FP_{sl}^{sv}$ data to the one calculated by the $FP_{sl}^{pv}$ method:

$$\Delta A_{\kappa}^{\mathrm{FP_{sl}^{pv}-ML}} = \int_0^1 \left\langle \frac{\partial H_{\kappa}^{\mathrm{FP_{sl}^{pv}-ML}}}{\partial \eta} \right\rangle_{\eta} d\eta, \tag{S4}$$

$$H_{\kappa}^{\mathrm{FP_{sl}^{pv}-ML}} = \sum_{i=1}^{N_\mathrm{a}} \frac{|\mathbf{p}_i|^2}{2m_i} + \eta U_{\kappa}^{\mathrm{FP_{sl}^{pv}}} + (1-\eta)\, U_{\kappa}^{\mathrm{ML}}, \tag{S5}$$

where the superscript 'ML' denotes the MLFF model trained on the $FP_{sl}^{sv}$ method similarly to Methods section in the main text. By using the abbreviations introduced in the main text, the TI simulation is written as ML(Ox) $\rightarrow$ $FP_{sl}^{pv}$(Ox) and ML(Red) $\rightarrow$ $FP_{sl}^{pv}$(Red). The free energy change of the redox potential $\Delta A^{\mathrm{FP_{sl}^{pv}}}$ is obtained as $\Delta A^{\mathrm{ML}} + \Delta A_1^{\mathrm{FP_{sl}^{pv}-ML}} - \Delta A_0^{\mathrm{FP_{sl}^{pv}-ML}}$. The other method is a direct TI simulation without any ML surrogate model from the oxidized state to the reduced state:

$$\Delta A^{\mathrm{FP_{sl}^{pv}}} = \int_0^1 \left\langle \frac{\partial H^{\mathrm{FP_{sl}^{pv}}}}{\partial \lambda} \right\rangle_{\lambda} d\lambda, \tag{S6}$$

$$H^{\mathrm{FP_{sl}^{pv}}} = \sum_{i=1}^{N_\mathrm{a}} \frac{|\mathbf{p}_i|^2}{2m_i} + \lambda U_1^{\mathrm{FP_{sl}^{pv}}} + (1-\lambda)\, U_0^{\mathrm{FP_{sl}^{pv}}} - Ne\Delta\bar{\phi}. \tag{S7}$$

The integration is represented as $FP_{sl}^{pv}$(Ox) $\rightarrow$ $FP_{sl}^{pv}$(Red).

The redox potential of the non-local hybrid functional was computed by the TPT calculation

Table S 8. Effects of semi-core electron relaxations on the redox potential (V vs. SHE) of the $Cu^{2+}/Cu^{+}$ couple. The notations in this table follows the ones in Fig. 4 in the main text.

| PAW type | $FP_{sl}$ (w/ ML) (RPBE+D3) | $FP_{sl}$ (w/o ML) RPBE+D3 | $FP_{nl}$ (w/ ML) [PBE0+D3 (0.25)] |
|---|---|---|---|
| sv ($3d^{10}4p^{1}$) | 0.66±0.05 | 0.69±0.07 | 0.24±0.07 |
| pv ($3p^{6}3d^{10}4p^{1}$) | 0.65±0.05 | 0.63±0.10 | 0.20±0.06 |

Table S 9. Effects of semi-core electron relaxations in Cu ions on the averaged value of 1s levels of oxygen atoms ($\langle \varepsilon_{1s,bulk} \rangle_{\lambda}$) at the region far from the redox species. Unit is in eV.

| | $FP_{sl}$ (RPBE+D3) | | $FP_{nl}$ [PBE0+D3 (0.25)] | |
|---|---|---|---|---|
| PAW type | $Cu^{2+}$+64$H_2O$ | $Cu^{+}$+64$H_2O$ | $Cu^{2+}$+64$H_2O$ | $Cu^{+}$+64$H_2O$ |
| sv ($3d^{10}4p^{1}$) | −507.50±0.01 | −507.47±0.01 | −507.51±0.01 | −507.52±0.01 |
| pv ($3p^{6}3d^{10}4p^{1}$) | −507.50±0.01 | −507.50±0.01 | −507.51±0.01 | −507.52±0.01 |

based on the trajectory of the $FP_{sl}^{sv}$ method:

$$\Delta A_{\kappa}^{FP_{nl}^{pv}-FP_{sl}^{sv}} \simeq \left\langle \Delta U_{\kappa}^{\Delta ML^{pv}} \right\rangle_{FP_{sl}^{sv}} - \frac{\beta}{2} \left\langle \left( \Delta U_{\kappa}^{\Delta ML^{pv}} - \left\langle \Delta U_{\kappa}^{\Delta ML^{pv}} \right\rangle_{FP_{sl}^{sv}} \right)^{2} \right\rangle_{FP_{sl}^{sv}}, \tag{S8}$$

where $\Delta U_{\kappa}^{\Delta ML^{pv}}$ represents the potential energy difference predicted by the Δ-ML model trained on the difference between the potential energy calculated by the $FP_{nl}^{pv}$ method and the one calculated by the $FP_{sl}^{sv}$ method. The free energy change for the $FP_{nl}^{pv}$ method is obtained as $\Delta A^{FP_{sl}^{sv}} + \Delta A_{1}^{FP_{nl}^{pv}-FP_{sl}^{sv}} - \Delta A_{0}^{FP_{nl}^{pv}-FP_{sl}^{sv}}$.

The calculated redox potentials are listed in Table S8. All relevant supporting data of the results are summarized in Fig. S15. The redox potential calculated by pv agrees with the one calculated by sv within the statistical error bars, indicating that the impacts of the semi-core electron relaxation are negligibly small in our PAW method.

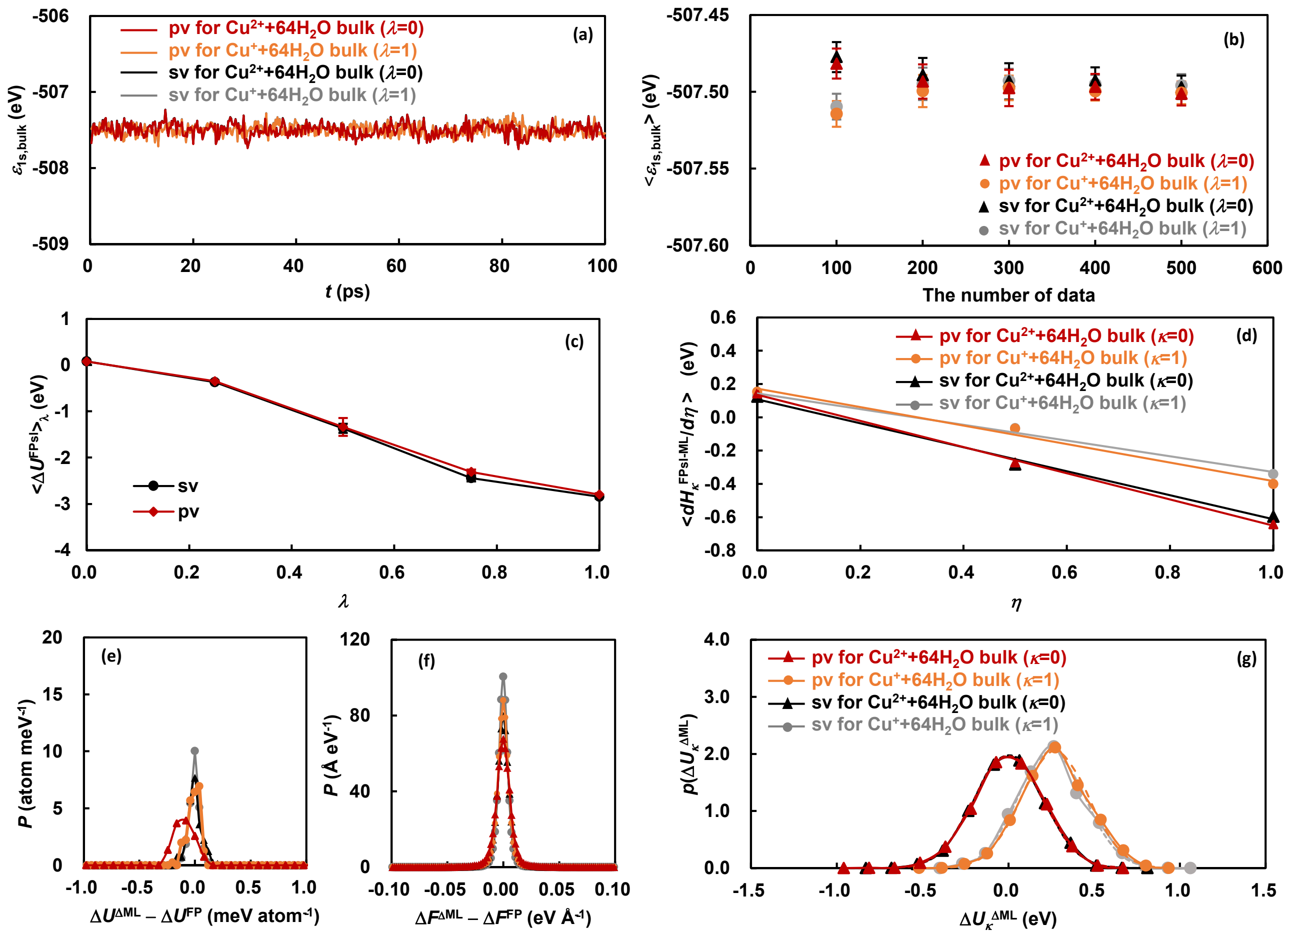


Figure S 15. Summary of data related to the redox potential of the $Cu^{2+}/Cu^{+}$ couple computed using the PAW with the electronic configuration of $3p^6 3d^{10} 4p^1$(pv): (a) time evolution of oxygen 1s ($\varepsilon_{1s,bulk}$) in the bulk solutions modeled by $Cu^{2+}$+64H2O and $Cu^{+}$+64H2O, (b) the averages of $\varepsilon_{1s,bulk}$ as functions of the number of structures, (c) the energy contribution $\langle \Delta U^{FP_{sl}} \rangle_\lambda = \left\langle U_1^{FP_{sl}} - U_0^{FP_{sl}} \right\rangle_\lambda$ from Eq. (S6) of the TI along the coupling parameter $\lambda$, using the RPBE+D3 functional ($FP_{sl}$ method) without any ML model, (d) integrands of Eq. (S4) of the TI along the coupling parameter $\eta$, (e, f) error distribution of the Δ-ML model for the test $FP_{nl}^{pv}$ data on 50 structures, and (g) probability distributions of energy differences $\Delta U_\kappa^{\Delta ML^{pv}}$ in the TPT calculations. Results for the PAW with the electronic configuration of ($3d^{10}4p^1$) (sv) are also shown for comparison.

## S8. NOTES ON GAUSSIAN AND LINEAR ASSUMPTIONS IN TPT

Here, we assume that the probability distribution of $\Delta U$ at $\lambda$ is Gaussian

$$p_\lambda(\Delta U) = \frac{1}{\sqrt{2\pi}\sigma}\exp\left[-\frac{(\Delta U - \langle\Delta U\rangle_\lambda)^2}{2\sigma^2}\right]. \tag{S9}$$

The expectation of $\exp(-\beta\Delta U)$ is derived as

$$\begin{aligned}\langle\exp(-\beta\Delta U)\rangle_\lambda &= \frac{1}{\sqrt{2\pi}\sigma} \\ &\times \int_{-\infty}^{+\infty}\exp(-\beta\Delta U) \\ &\times \exp\left[-\frac{(\Delta U - \langle\Delta U\rangle_\lambda)^2}{2\sigma^2}\right] d\Delta U \\ &= \langle\exp(-\beta\Delta U)\rangle_\lambda \exp\left[\frac{1}{2}(\sigma\beta)^2\right].\end{aligned} \tag{S10}$$

Similarly, the expectation of $\exp(\beta\Delta U)$ is derived as

$$\langle\exp(\beta\Delta U)\rangle_\lambda = \exp(\beta\langle\Delta U\rangle_\lambda)\exp\left[\frac{1}{2}(\sigma\beta)^2\right]. \tag{S11}$$

Since $\sigma^2 = \left\langle(\Delta U - \langle\Delta U\rangle_\lambda)^2\right\rangle_\lambda$, the free energy difference $\Delta F$ is derived as

$$\begin{aligned}\Delta F &= \langle\Delta U\rangle_0 - \frac{\beta}{2}\left\langle(\Delta U - \langle\Delta U\rangle_0)^2\right\rangle_0 \\ &= \langle\Delta U\rangle_1 + \frac{\beta}{2}\left\langle(\Delta U - \langle\Delta U\rangle_1)^2\right\rangle_1.\end{aligned} \tag{S12}$$

The Gaussian assumption also leads to the linearity of the integrand in Eq. (2) in the main text. The integrand of Eq. (2) is written as

$$\begin{aligned}I(\lambda) &= \langle\Delta U\rangle_\lambda \\ &= \frac{\int d\mathbf{R}\Delta U\exp[-\beta(\lambda U_1 + (1-\lambda)U_0)]}{\int d\mathbf{R}\exp[-\beta(\lambda U_1 + (1-\lambda)U_0)]}.\end{aligned} \tag{S13}$$

The first derivative of the integrand with respect to the coupling parameter $\lambda$ is

$$\begin{aligned}
\left.\frac{dI}{d\lambda}\right|_{\lambda} &= -\beta \frac{\int d\mathbf{R}\Delta U^2 \exp\left[-\beta\left(\lambda U_1 + (1-\lambda) U_0\right)\right]}{\int d\mathbf{R} \exp\left[-\beta\left(\lambda U_1 + (1-\lambda) U_0\right)\right]} \\
&\quad + \beta \left(\frac{\int d\mathbf{R}\Delta U \exp\left[-\beta\left(\lambda U_1 + (1-\lambda) U_0\right)\right]}{\int d\mathbf{R} \exp\left[-\beta\left(\lambda U_1 + (1-\lambda) U_0\right)\right]}\right)^2 \\
&= -\beta \left(\left\langle \Delta U^2 \right\rangle_{\lambda} - \left\langle \Delta U \right\rangle_{\lambda}^2\right) \\
&= -\beta \left\langle \left(\Delta U - \left\langle \Delta U \right\rangle_{\lambda}\right)^2 \right\rangle_{\lambda}.
\end{aligned} \tag{S14}$$

Here, we assume that $I(\lambda)$ is a linear function of $\lambda$. This implies the following equations:

$$\begin{aligned}
I(\lambda) &= I(0) + \lambda \left.\frac{dI}{d\lambda}\right|_0 \\
&= I(1) + (1-\lambda) \left.\frac{dI}{d\lambda}\right|_1,
\end{aligned} \tag{S15}$$

$$\left.\frac{dI}{d\lambda}\right|_0 = \left.\frac{dI}{d\lambda}\right|_1. \tag{S16}$$

Substituting Eq. (S15) into the TI gives Eq. (S11), indicating that the linear assumption [Eqs. (S15) and (S16)] leads to the condition derived from the Gaussian assumption.

Another noticeable point is that the first derivative of the integrand equals to the variance of the Gaussian distribution as indicated by Eq. (S14). The relation is observed in the TI calculations using the MLFF and FP method as shown in Section S4.

## S9. LEARNING CURVES OF MLFF AND Δ-ML MODELS AND ACCURACY OF REDOX POTENTIALS PREDICTED BY MLFF MODELS

Figure S16 shows the redox potential $U_{\mathrm{redox}}$ predicted by the MLFF models trained using the RPBE+D3 functional ($\mathrm{FP_{sl}}$ method) as a function of the number $N_{\mathrm{st}}$ of structures providing the training data. Root mean square errors (RMSEs) of energies and forces predicted by the MLFF models are also presented. Here, the number of training data was increased by decreasing the threshold for the spilling factor, which was used to judge the necessity of the FP data sampling during the on-the-fly training, from 0.02 to 0.001. As $N_{\mathrm{st}}$ increases, RMSEs decrease, and $U_{\mathrm{redox}}$ approaches to the one predicted by the $\mathrm{FP_{sl}}$ method. However, because of limitations in the descriptors and energy representations of the MLFFs, there is a limit to the improvement in accuracy that can be achieved by increasing the amount of data. Therefore, we consider that corrections through the TI and TPT calculations are necessary. Because the TI and TPT corrections are judged to be necessary for all MLFF models, we used the MLFF models with the smallest data size shown in Fig. S16.

Figure S17 shows the learning curves for the Δ-ML models trained on differences in energies and forces between the PBE0 (0.25) functional and RPBE+D3 functional. High accuracy is already achieved by the models training on merely 10 structures. Very similar results were obtained also for other functionals (not shown because of a lot of similarity).

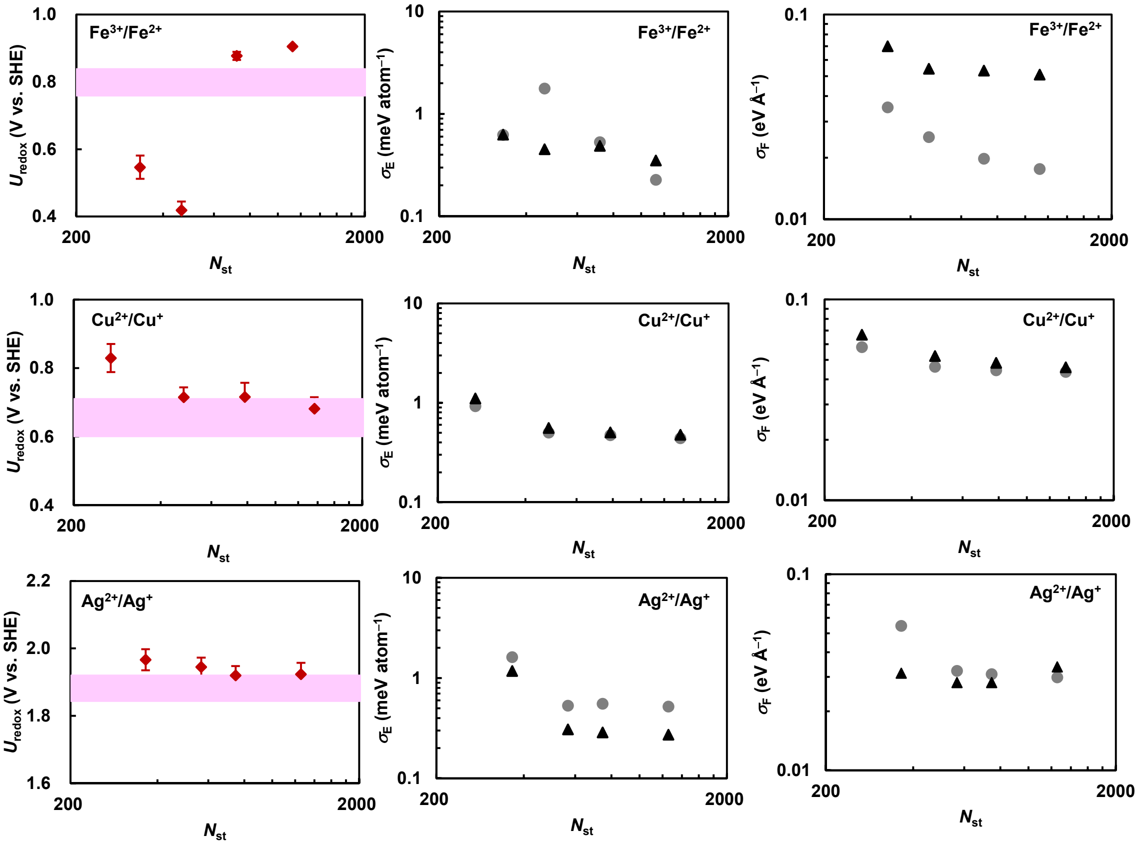


Figure S 16. Redox potential $U_{\mathrm{redox}}$ predicted by MLFF models trained using the RPBE+D3 functional ($FP_{\mathrm{sl}}$ method) is presented as a function of the number $N_{\mathrm{st}}$ of structures providing the training data. The light pink horizontal lines indicate $U_{\mathrm{redox}}$ calculated by the $FP_{\mathrm{sl}}$ method. The thickness of these lines represents the statistical uncertainty. RMSEs of energies and forces for the oxidized states (black triangles) and the reduced states (gray circles) are also shown for comparison. Here, $N_{\mathrm{st}}$ is a sum of the numbers of structures for the oxidized and reduced states.

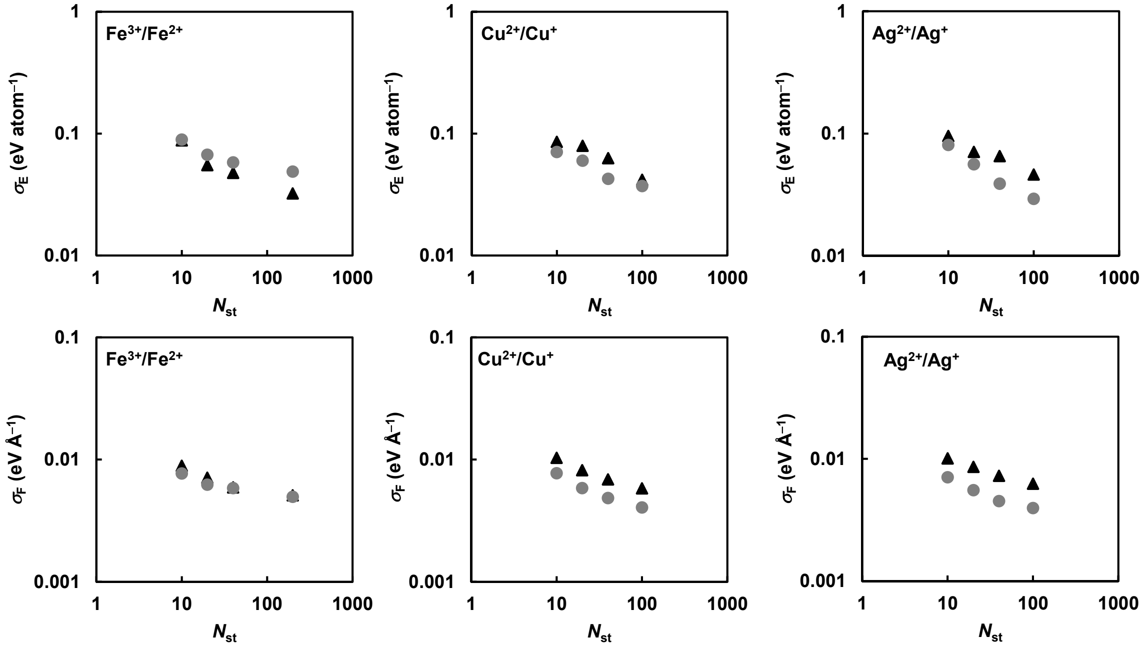


Figure S 17. Learning curves [RMSEs for energies ($\sigma_{\mathrm{E}}$) and forces ($\sigma_{\mathrm{F}}$) vs. the number $N_{\mathrm{st}}$ of structures providing the training data] for Δ-ML models trained on differences in energies and forces between the PBE0 (0.25) functional and RPBE+D3 functional.

[1] M. P. Allen and D. J. Tildesley. *Computer Simulation of Liquids*. 1987.

[2] S. Trasatti. The absolute electrode potential: an explanatory note (recommendations 1986). *Pure and Applied Chemistry*, 58(7):955–966, 1986.

[3] A.J. Bard, R. Parsons, and J. Jordan. *Standard Potentials in Aqueous Solution*. Monographs in Electroanalytical Chemistry and Electrochemistr. Taylor & Francis, 1985.

[4] Jiabo Le, Marcella Iannuzzi, Angel Cuesta, and Jun Cheng. Determining potentials of zero charge of metal electrodes versus the standard hydrogen electrode from density-functional-theory-based molecular dynamics. *Phys. Rev. Lett.*, 119:016801, Jul 2017.
